# Supplementary material for: Mean-Field Approximation of Dynamics on Networks
Source: arXiv:2508.16304 source file (2025-08-22)
Supplement: Supplementary file 1 [file SI.pdf]

# SUPPLEMENTARY MATERIALS: MEAN-FIELD APPROXIMATION OF DYNAMICS ON NETWORKS*

JONATHAN A. WARD[†], GÁBOR TIMÁR[†], AND PÉTER L. SIMON[‡]

**SM1. Introduction.** Sections SM2 to SM5 of this document are intended to supplement Sections 2 to 5 in the main paper with an illustrative example. The sections here could be read alongside those in the main paper or separately, although the general theory presented here is highly abbreviated.

**SM2. Mathematical background.** Let $G = (V, E)$ denote a network with vertex set $V$ and edge set $E \subset V \times V$, where the number of vertices is $N = |V|$. Unless otherwise stated, we consider dynamical processes on finite simple networks (i.e. undirected, unweighted with no self-loops or multiple edges) described by continuous-time Markov chains where each vertex can be in one of a finite number $M$ of *vertex-states* and the set of possible vertex-states is $\mathcal{W} = \{\mathcal{W}_1, \mathcal{W}_2, \ldots, \mathcal{W}_M\}$.

**SM2.1. State-space.** The state-space of the Markov chain is the set of all permutations of $N$ vertex-states chosen from $\mathcal{W}$ with repetition. This is equivalent to $\mathcal{S} = \mathcal{W}^V$, i.e. the set of all functions from $V$ to $\mathcal{W}$, and so if the network is in state $S \in \mathcal{S}$ then the vertex-state of vertex $v \in V$ is $S(v)$. We refer to the states $S \in \mathcal{S}$ as *microstates* and the number of microstates in $\mathcal{S}$ is $M^N$. We enumerate the microstates as $\mathcal{S} = \{S^{[1]}, S^{[2]}, \ldots, S^{[M^N]}\}$.

As an illustration of the theory developed in the main paper, a simple example will be presented here, specifically for dynamics on a square/two-by-two lattice/four cycle with vertices $V = \{1, 2, 3, 4\}$, illustrated in Figure SM1. We will refer to this as the square example. In this example, we consider SISa dynamics in which vertices are either susceptible, which corresponds to $\mathcal{W}_1 = \mathcal{B}$ and the colour blue, or infected, which corresponds to $\mathcal{W}_2 = \mathcal{R}$ and the colour red. The total number of microstates is $M^N = 2^4 = 16$, we number them as illustrated in Figure SM2.

**SM2.2. Transitions.** We assume that changes in microstate correspond to a single vertex $v \in V$ changing its vertex-state, and the rate that this occurs is a function of only the number of $v$'s neighbours in each of the vertex-states. We also assume that this rate function is the same for all vertices. In the models we consider, $\mathbf{R}_{\mathcal{A},\mathcal{B}}(n_1, n_2, \ldots, n_M) \geq 0$ gives the rate that a vertex in vertex-state $\mathcal{A}$ changes to vertex-state $\mathcal{B}$ if it has $n_1$ neighbours in vertex-state $\mathcal{W}_1$, $n_2$ neighbours in vertex-state $\mathcal{W}_2$, etc. If transitions between a pair of vertex-states $\mathcal{A}, \mathcal{B} \in \mathcal{W}$ do not occur in a particular model, then the rate $\mathbf{R}_{\mathcal{A},\mathcal{B}}$ is identically zero. We consider models where $\mathbf{R}_{\mathcal{A},\mathcal{B}}$ is an affine function, i.e.

$$\mathbf{R}_{\mathcal{A},\mathcal{B}}(n_1, n_2, \ldots, n_M) = \zeta_0^{\mathcal{A},\mathcal{B}} + \sum_{m=1}^{M} \zeta_m^{\mathcal{A},\mathcal{B}} n_m, \tag{SM2.1}$$

To illustrate the transitions between microstates, consider the example of SISa dynamics. A susceptible vertex $v$ with $n_1$ susceptible neighbours and $n_2$ infected

*Submitted to the editors DATE.

**Funding:** J.A. Ward and G. Timár acknowledge funding from the Leverhulme Trust Project Grant number RPG-2023-187. P.L. Simon acknowledges support from the Hungarian Scientific Research Fund, OTKA (grant no. 135241) and from ERC Synergy Grant No. 810115 - DYNASNET.

[†]University of Leeds, UK (j.a.ward@leeds.ac.uk).

[‡]Eotvos Lorand University, Hungary

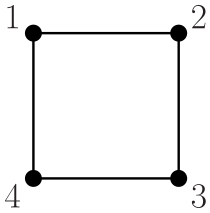


FIG. SM1. *Four cycle with vertex labelling.*

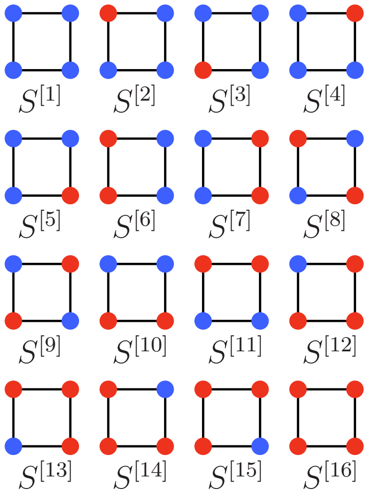


FIG. SM2. *Labelling of microstate-space, blue corresponds to susceptible and red to infected vertices.*

neighbours becomes infected at a rate $\alpha + \beta n_2$, where $\alpha, \beta > 0$, so

$$\mathbf{R}_{\mathcal{B},\mathcal{R}}(n_1, n_2) = \alpha + \beta n_2.$$

Thus $\zeta_0^{\mathcal{B},\mathcal{R}} = \alpha$, $\zeta_1^{\mathcal{B},\mathcal{R}} = 0$ and $\zeta_2^{\mathcal{B},\mathcal{R}} = \beta$. An infected vertex with $n_1$ susceptible neighbours and $n_2$ infected neighbours becomes susceptible at a rate $\gamma > 0$, so

$$\mathbf{R}_{\mathcal{R},\mathcal{B}}(n_1, n_2) = \gamma.$$

Thus $\zeta_0^{\mathcal{R},\mathcal{B}} = \gamma$ and $\zeta_1^{\mathcal{R},\mathcal{B}} = \zeta_2^{\mathcal{R},\mathcal{B}} = 0$.

**SM2.3. Kolmogorov equations: infinitesimal generator.** Let

$$X(t) = (X_1(t), X_2(t), \dots, X_{M^N}(t))^{\mathrm{T}}$$

be the time-dependent Markov chain probability distribution over $\mathcal{S}$, where $X_i(t)$ is the probability of being in microstate $S^{[i]}$ at time $t$. The evolution of $X(t)$ is then given by the forward Kolmogorov or master equation [SM4],

$$\dot{X} = \mathbf{Q}^{\mathrm{T}} X,$$

where $\mathbf{Q}$ is the infinitesimal generator, an $M^N$ by $M^N$ matrix in which each off-diagonal component $\mathbf{Q}_{kl}$ gives the transition rate from $S^{[k]}$ to $S^{[l]}$, and the diagonal components ensure that rows sum to zero so that probability is conserved. We assume that a vertex changes vertex-state instantaneously, thus transitions only occur between pairs of microstates that differ in exactly one vertex-state.

Considering the SISa dynamics on the square again, we can easily determine the entries of the matrix $\mathbf{Q}$. For example, $\mathbf{Q}_{9,12} = \alpha + 2\beta$, because the transition from $S^{[9]}$ to $S^{[12]}$ means that node 3 becomes infected. (See the numbering of nodes and states in Figures SM1 and SM2.) This can happen at rate $\alpha$ spontaneously and at rate $2\beta$ by infection along edges from nodes 2 and 4. Calculating the rates for all possible transition pairs, the infinitesimal generator of the small example is a $16 \times 16$ matrix that can be written as

$$\mathbf{Q} = \begin{pmatrix} \Delta_0 & \mathbf{A}_0 & 0 & 0 & 0 \\ \mathbf{B}_1 & \Delta_1 & \mathbf{A}_1 & 0 & 0 \\ 0 & \mathbf{B}_2 & \Delta_2 & \mathbf{A}_2 & 0 \\ 0 & 0 & \mathbf{B}_3 & \Delta_3 & \mathbf{A}_3 \\ 0 & 0 & 0 & \mathbf{B}_4 & \Delta_4 \end{pmatrix} \tag{SM2.2}$$

where the matrix $\mathbf{A}_k$ corresponds to infection from states with $k$ infected nodes, matrix $\mathbf{B}_k$ corresponds to recovery from states with $k$ infected nodes and the matrix $\Delta_k$ is diagonal with negative entries in the diagonal, determined in such a way that the sum of entries in a row of $Q$ is zero. These matrices take the following form:

$$\mathbf{A}_0 = \begin{pmatrix} \alpha & \alpha & \alpha & \alpha \end{pmatrix}, \quad \mathbf{A}_1 = \begin{pmatrix} \alpha+\beta & 0 & \alpha & 0 & 0 & \alpha+\beta \\ \alpha+\beta & 0 & 0 & \alpha & \alpha+\beta & 0 \\ 0 & \alpha+\beta & 0 & \alpha & 0 & \alpha+\beta \\ 0 & \alpha+\beta & \alpha & 0 & \alpha+\beta & 0 \end{pmatrix},$$

$$\mathbf{A}_2 = \begin{pmatrix} 0 & 0 & \alpha+\beta & \alpha+\beta \\ \alpha+\beta & \alpha+\beta & 0 & 0 \\ 0 & \alpha+2\beta & \alpha+2\beta & 0 \\ \alpha+2\beta & 0 & 0 & \alpha+2\beta \\ \alpha+\beta & 0 & \alpha+\beta & 0 \\ 0 & \alpha+\beta & 0 & \alpha+\beta \end{pmatrix}, \quad \mathbf{A}_3 = \begin{pmatrix} \alpha+2\beta \\ \alpha+2\beta \\ \alpha+2\beta \\ \alpha+2\beta \end{pmatrix},$$

$$\mathbf{B}_1 = \begin{pmatrix} \gamma \\ \gamma \\ \gamma \\ \gamma \end{pmatrix}, \quad \mathbf{B}_2 = \begin{pmatrix} \gamma & \gamma & 0 & 0 \\ 0 & 0 & \gamma & \gamma \\ \gamma & 0 & 0 & \gamma \\ 0 & \gamma & \gamma & 0 \\ 0 & \gamma & 0 & \gamma \\ \gamma & 0 & \gamma & 0 \end{pmatrix}, \quad \mathbf{B}_3 = \begin{pmatrix} 0 & \gamma & 0 & \gamma & \gamma & 0 \\ 0 & \gamma & \gamma & 0 & 0 & \gamma \\ \gamma & 0 & \gamma & 0 & \gamma & 0 \\ \gamma & 0 & 0 & \gamma & 0 & \gamma \end{pmatrix},$$

$$\mathbf{B}_4 = \begin{pmatrix} \gamma & \gamma & \gamma & \gamma \end{pmatrix}.$$

**SM3. Coarse-graining via lumping: theoretical foundation.** We consider *lumping* of Markov chains [SM3]. Let $\Pi_{\mathcal{S}} = \{\mathcal{S}_1, \mathcal{S}_2, \dots, \mathcal{S}_n\}$ be a partition of microstate-space, so $\mathcal{S}_i \cap \mathcal{S}_j = \emptyset$ for each $i \neq j$, and $\cup_i \mathcal{S}_i = \mathcal{S}$. We will refer to $\mathcal{S}_i$ as a *lumped state*. An *exact lumping* is a partition of microstate-space $\Pi_{\mathcal{S}}$ that preserves the Markov property, a necessary and sufficient condition for which is that the sum of transition rates out of a microstate $S^{[k]} \in \mathcal{S}_i$ into the cell $\mathcal{S}_j$ is the same

for all microstates in the cell $\mathcal{S}_i$. In matrix notation [SM6], this is equivalent to the existence of an $n \times n$ matrix $\mathbf{q}$ such that

$$\mathbf{QC} = \mathbf{Cq}, \tag{SM3.1}$$

where $\mathbf{C} \in \{0,1\}^{M^N \times n}$ is the *collector matrix* [SM2] whose $kj$th component is

$$\mathbf{C}_{kj} = \begin{cases} 1 & \text{if } S^{[k]} \in \mathcal{S}_j, \\ 0 & \text{otherwise,} \end{cases} \tag{SM3.2}$$

that is the collector matrix collects those microstates in a coloumn that belong to the same cell, or in other words, the same macro-state, in the partition. We call (SM3.1) the *lumpability condition.*

Note that $\mathbf{q}$ can be given explicitly for an exact lumping by introducing the *distributor matrix* [SM2] $\mathbf{D} \in \mathbb{R}^{n \times M^N}$, whose $il$th component is

$$\mathbf{D}_{il} = \begin{cases} \frac{1}{|\mathcal{S}_i|} & \text{if } S^{[l]} \in \mathcal{S}_i, \\ 0 & \text{otherwise.} \end{cases} \tag{SM3.3}$$

Specifically, $\Pi_{\mathcal{S}}$ satisfies the lumpability condition when $\mathbf{Q}$ commutes with $\mathbf{CD}$ [SM6]. Note that $\mathbf{DC} = \mathbf{I}$, the identity matrix, hence multiplying (SM3.1) by $\mathbf{D}$ we get the generator $\mathbf{q}$ of the lumped system explicitly as

$$\mathbf{q} = \mathbf{DQC}. \tag{SM3.4}$$

A lumping that does not satisfy the lumpability condition is an *approximate lumping* [SM2]. Given a partition $\Pi_{\mathcal{S}}$ of microstate-space that does not satisfy the lumpability condition (SM3.1), our approach is to still use the set of lumped states $\Pi_{\mathcal{S}}$ and the corresponding generator $\mathbf{q} = \mathbf{DQC}$. Summarising, we can say that starting from the full infinitesimal generator, $\mathbf{Q}$, and choosing a partition of the state-space, equation (**??**) yields the infinitesimal generator $\mathbf{q}$ of the lumped (coarse-grained) system. Note that the partition of the state-space is encoded in the collector and distributor matrices, $\mathbf{C}$ and $\mathbf{D}$ respectively.

**SM4. Lumping based on vertex set partitions.** In the previous section we introduced the notion of lumping in general. In this section we illustrate how a partition of vertices is used to partition the microstate-space.

**SM4.1. State-space partition based on a vertex set partition.** Given a partition of the *vertex* set, we consider lumped states based on a partition of microstate-space into sets of microstates with the same number of vertices in each vertex-state *within* each of the cells of the *vertex* partition.

Let us consider an SISa epidemic propagating on a square graph. In this example we consider a two cell partition of vertices $\Pi_V = \{V_1, V_2\}$, where $V_1 = \{1, 4\}$ and $V_2 = \{2, 3\}$. Crucially, this choice of vertex partition allows us to illustrate an example of an approximate lumping[1]. We use $N_1 = |V_1|$ and $N_2 = |V_2|$ to denote the number of vertices in $V_1$ and $V_2$ respectively, so $N_1 = N_2 = 2$, and we use $P = 2$ to denote the number of vertex-partition cells. We will keep our notation general in this example, e.g. by using $P$ rather than 2, where it does not add excessive complexity. Our approximate lumping will be based on the number of susceptible and infected vertices

[1] Note however that in this example it is possible to obtain an exact lumping by choosing vertices in opposite corners to be in the same cell of the vertex partition.

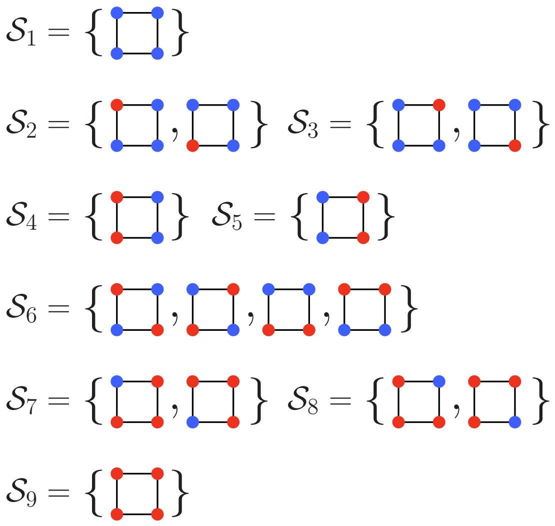


FIG. SM3. *Approximate lumping partition of microstate-space for the square example.*

in each of the cells in the vertex-partition. We will thus use a two-by-two matrix to represent lumped states, where the rows correspond to vertex-states (susceptible, infected) and the columns correspond to the partition cells ($V_1$ and $V_2$). Specifically, lumped states will be denoted by $\mathbf{s} \in \mathbb{Z}_{\geq 0}^{M \times P}$, a two-by-two matrix of non-negative integers whose $m,p$th entry, $\mathbf{s}_{m,p}$, is the number of vertices in vertex-state $\mathcal{W}_m$ in the vertex partition cell $V_p$. Note that $\mathbf{s}_{1,p} + \mathbf{s}_{2,p} = N_p$ for $p = 1, 2$ and adding these for $p = 1$ and $p = 2$ we get that the sum of the entries in a matrix $\mathbf{s}$ is $N_1 + N_2 = N = 4$.

**SM4.2. The size of the lumped state-space and the sizes of the partition cells.** Since there are $N_1 = 2$ vertices in the first partition cell and $M = 2$ vertex states, the possible values for $\mathbf{s}_{1,1}$ are 0, 1 and 2. The corresponding values for $\mathbf{s}_{2,1}$ are 2, 1 and 0 respectively, since $\mathbf{s}_{1,1} + \mathbf{s}_{2,1} = N_p = 2$. These three possibilities arise because a lumped state corresponds to choosing $N_1$ vertices from the $M$ possible vertex-states with repetition, which is $\binom{N_1+M-1}{N_1}$. A similar argument applies to the second partition cell and hence the total number of lumped states is

$$n = \binom{N_1 + M - 1}{N_1}\binom{N_2 + M - 1}{N_2} = \binom{3}{2}\binom{3}{2} = 9, \tag{SM4.1}$$

and we label these as follows:

$$\mathbf{s}^{[1]} = \begin{pmatrix} 2 & 2 \\ 0 & 0 \end{pmatrix}, \mathbf{s}^{[2]} = \begin{pmatrix} 1 & 2 \\ 1 & 0 \end{pmatrix}, \mathbf{s}^{[3]} = \begin{pmatrix} 2 & 1 \\ 0 & 1 \end{pmatrix},$$
$$\mathbf{s}^{[4]} = \begin{pmatrix} 0 & 2 \\ 2 & 0 \end{pmatrix}, \mathbf{s}^{[5]} = \begin{pmatrix} 2 & 0 \\ 0 & 2 \end{pmatrix}, \mathbf{s}^{[6]} = \begin{pmatrix} 1 & 1 \\ 1 & 1 \end{pmatrix},$$
$$\mathbf{s}^{[7]} = \begin{pmatrix} 1 & 0 \\ 1 & 2 \end{pmatrix}, \mathbf{s}^{[8]} = \begin{pmatrix} 0 & 1 \\ 2 & 1 \end{pmatrix}, \mathbf{s}^{[9]} = \begin{pmatrix} 0 & 0 \\ 2 & 2 \end{pmatrix}.$$

The corresponding vertex-partition approximate lumping $\Pi_{\mathcal{S}} = \{\mathcal{S}_1, \mathcal{S}_2, \ldots, \mathcal{S}_9\}$ is illustrated in Figure SM3. For example, there is one microstate in $\mathcal{S}^{[1]}$ (which cor-

responds to $\mathbf{s}^{[1]}$) which has 2 susceptible (blue) vertices in both $V_1$ (vertices on the left of the square) and $V_2$ (vertices on the right of the square), and no infected (red) vertices in either vertex partition cell. Similarly, microstates in $\mathcal{S}^{[8]}$ have two infected vertices in $V_1$ and both a susceptible and an infected vertex in $V_2$.

The number of microstates that correspond to $\mathbf{s}^{[i]}$ is equivalent to the number of ways to choose $\mathbf{s}^{[i]}_{1,1}$ susceptible vertices in the first partition, multiplied by the number of ways to choose $\mathbf{s}^{[i]}_{1,2}$ susceptible vertices in the second partition. As a notational short-hand, we will use

$$\binom{N}{\mathbf{s}^{[i]}} := \binom{N_1}{\mathbf{s}^{[i]}_{1,1}}\binom{N_2}{\mathbf{s}^{[i]}_{1,2}} = \frac{N_1!}{\mathbf{s}^{[i]}_{1,1}!\,\mathbf{s}^{[i]}_{2,1}!} \times \frac{N_2!}{\mathbf{s}^{[i]}_{2,1}!\,\mathbf{s}^{[i]}_{2,2}!},$$

thus for our square example we have

$$\begin{aligned}
&\binom{N}{\mathbf{s}^{[1]}} = \binom{2}{2}\binom{2}{2} = 1, \quad \binom{N}{\mathbf{s}^{[2]}} = \binom{N}{\mathbf{s}^{[3]}} = \binom{2}{1}\binom{2}{2} = 2,\\
&\binom{N}{\mathbf{s}^{[4]}} = \binom{N}{\mathbf{s}^{[5]}} = \binom{2}{0}\binom{2}{2} = 1, \quad \binom{N}{\mathbf{s}^{[6]}} = \binom{2}{1}\binom{2}{1} = 4,\\
&\binom{N}{\mathbf{s}^{[7]}} = \binom{N}{\mathbf{s}^{[8]}} = \binom{2}{1}\binom{2}{2} = 2, \quad \text{and} \binom{N}{\mathbf{s}^{[9]}} = \binom{2}{0}\binom{2}{0} = 1.
\end{aligned}$$

**SM4.3. Lumped generator for the square SISa example.** Now we compute the infinitesimal generator for the example with SISa epidemic on a square network based on equation (SM3.4).

The collector matrix, $\mathbf{C}$, for our approximate lumping of the square is a matrix of size $16 \times 9$, with most of the entries zeros and one entry in each row which is 1. The element in the $k$-th row is $\mathbf{C}_{kj}$ if the microstate $S^{[k]}$ belongs to the lumped state $\mathcal{S}_j$. Based on the labelling of the states in Figure SM2 and those of the lumping classes given in Figure SM3, the non-zero entries of the collector matrix are

$$\mathbf{C}_{1,1}, \mathbf{C}_{2,2}, \mathbf{C}_{3,2}, \mathbf{C}_{4,3}, \mathbf{C}_{5,3}, \mathbf{C}_{6,4}, \mathbf{C}_{7,5}, \mathbf{C}_{8,6}, \mathbf{C}_{9,6},$$
$$\mathbf{C}_{10,6}, \mathbf{C}_{11,6}, \mathbf{C}_{12,7}, \mathbf{C}_{13,7}, \mathbf{C}_{14,8}, \mathbf{C}_{15,8}, \mathbf{C}_{16,9}.$$

The matrix $\mathbf{C}$ has a block diagonal form

$$\mathbf{C} = \begin{pmatrix} \mathbf{C}_0 & 0 & 0 & 0 & 0 \\ 0 & \mathbf{C}_1 & 0 & 0 & 0 \\ 0 & 0 & \mathbf{C}_2 & 0 & 0 \\ 0 & 0 & 0 & \mathbf{C}_3 & 0 \\ 0 & 0 & 0 & 0 & \mathbf{C}_4 \end{pmatrix}$$

with $\mathbf{C}_0 = (1) = \mathbf{C}_4$ and

$$\mathbf{C}_1 = \mathbf{C}_3 = \begin{pmatrix} 1 & 0 \\ 1 & 0 \\ 0 & 1 \\ 0 & 1 \end{pmatrix}, \quad \mathbf{C}_2 = \begin{pmatrix} 1 & 0 & 0 \\ 0 & 1 & 0 \\ 0 & 0 & 1 \\ 0 & 0 & 1 \\ 0 & 0 & 1 \\ 0 & 0 & 1 \end{pmatrix}.$$

Note that this choice of blocks does not correspond to the lumped states, rather it relates to the number of infected vertices and the block tri-diagonal structure of $\mathbf{Q}$

seen in (SM2.2). Multiplying the infinitesimal generator $\mathbf{Q}$ by $\mathbf{C}$ we get the block tri-diagonal form

$$\text{(SM4.2)} \qquad \mathbf{QC} = \begin{pmatrix} \Delta_0\mathbf{C}_0 & \mathbf{A}_0\mathbf{C}_1 & 0 & 0 & 0 \\ \mathbf{B}_1\mathbf{C}_0 & \Delta_1\mathbf{C}_1 & \mathbf{A}_1\mathbf{C}_2 & 0 & 0 \\ 0 & \mathbf{B}_2\mathbf{C}_1 & \Delta_2\mathbf{C}_2 & \mathbf{A}_2\mathbf{C}_3 & 0 \\ 0 & 0 & \mathbf{B}_3\mathbf{C}_2 & \Delta_3\mathbf{C}_3 & \mathbf{A}_3\mathbf{C}_4 \\ 0 & 0 & 0 & \mathbf{B}_4\mathbf{C}_3 & \Delta_4\mathbf{C}_4 \end{pmatrix}$$

Each block can be easily calculated, we show only

$$\mathbf{A}_2\mathbf{C}_3 = \begin{pmatrix} 0 & 2\alpha+\beta \\ 2\alpha+\beta & 0 \\ \alpha+2\beta & \alpha+2\beta \\ \alpha+2\beta & \alpha+2\beta \\ \alpha+\beta & \alpha+\beta \\ \alpha+\beta & \alpha+\beta \end{pmatrix}$$

which shows that this lumping is not exact. Namely, recall that a lumping is exact if the total rate from a microstate $S^{[k]} \in \mathcal{S}_i$ into a lumped state $\mathcal{S}_j$ is the same for all microstates in $\mathcal{S}_i$. In the expression for $\mathbf{QC}$ above, there are two lumped transitions where this is not the case, namely from $\mathcal{S}_6$ to $\mathcal{S}_7$ (rows 3 to 6 in the first column of the matrix $\mathbf{A}_2\mathbf{C}_3$), and from $\mathcal{S}_6$ to $\mathcal{S}_8$ (rows 3 to 6 in the second column of this matrix). In both cases, there are two microstates where the rate is $\alpha + 2\beta$ and two where it is $\alpha + \beta$. This confirms that our partition of vertices is an approximate lumping.

We will now compute the lumped transition rate. The distributor matrix has the block diagonal form

$$\mathbf{D} = \begin{pmatrix} \mathbf{D}_0 & 0 & 0 & 0 & 0 \\ 0 & \mathbf{D}_1 & 0 & 0 & 0 \\ 0 & 0 & \mathbf{D}_2 & 0 & 0 \\ 0 & 0 & 0 & \mathbf{D}_3 & 0 \\ 0 & 0 & 0 & 0 & \mathbf{D}_4 \end{pmatrix}$$

with $\mathbf{D}_0 = (1) = \mathbf{D}_4$ and

$$\mathbf{D}_1 = \mathbf{D}_3 = \begin{pmatrix} \frac{1}{2} & \frac{1}{2} & 0 & 0 \\ 0 & 0 & \frac{1}{2} & \frac{1}{2} \end{pmatrix}, \quad \mathbf{D}_2 = \begin{pmatrix} 1 & 0 & 0 & 0 & 0 & 0 \\ 0 & 1 & 0 & 0 & 0 & 0 \\ 0 & 0 & \frac{1}{4} & \frac{1}{4} & \frac{1}{4} & \frac{1}{4} \end{pmatrix}.$$

Again, this choice of blocks does not reflect the lumping partition. Multiplying $\mathbf{QC}$, given in (SM4.2), by $\mathbf{D}$ we get $\mathbf{q}$ in the block tri-diagonal form

(SM4.3)

$$\mathbf{q} = \mathbf{DQC} = \begin{pmatrix} \mathbf{D}_0\Delta_0\mathbf{C}_0 & \mathbf{D}_0\mathbf{A}_0\mathbf{C}_1 & 0 & 0 & 0 \\ \mathbf{D}_1\mathbf{B}_1\mathbf{C}_0 & \mathbf{D}_1\Delta_1\mathbf{C}_1 & \mathbf{D}_1\mathbf{A}_1\mathbf{C}_2 & 0 & 0 \\ 0 & \mathbf{D}_2\mathbf{B}_2\mathbf{C}_1 & \mathbf{D}_2\Delta_2\mathbf{C}_2 & \mathbf{D}_2\mathbf{A}_2\mathbf{C}_3 & 0 \\ 0 & 0 & \mathbf{D}_3\mathbf{B}_3\mathbf{C}_2 & \mathbf{D}_3\Delta_3\mathbf{C}_3 & \mathbf{D}_3\mathbf{A}_3\mathbf{C}_4 \\ 0 & 0 & 0 & \mathbf{D}_4\mathbf{B}_4\mathbf{C}_3 & \mathbf{D}_4\Delta_4\mathbf{C}_4 \end{pmatrix}.$$

Each block can be easily calculated, and hence the coarsegrained approximate lumping

infinitesimal generator is

(SM4.4)

$$\mathbf{q} = \left(\begin{array}{c|cc|ccc|cc|c} \delta_1 & 2\alpha & 2\alpha & 0 & 0 & 0 & 0 & 0 & 0 \\ \hline \gamma & \delta_2 & 0 & \alpha+\beta & 0 & 2\alpha+\beta & 0 & 0 & 0 \\ \gamma & 0 & \delta_3 & 0 & \alpha+\beta & 2\alpha+\beta & 0 & 0 & 0 \\ \hline 0 & 2\gamma & 0 & \delta_4 & 0 & 0 & 0 & 2(\alpha+\beta) & 0 \\ 0 & 0 & 2\gamma & 0 & \delta_5 & 0 & 2(\alpha+\beta) & 0 & 0 \\ 0 & \gamma & \gamma & 0 & 0 & \delta_6 & \alpha+\frac{3}{2}\beta & \alpha+\frac{3}{2}\beta & 0 \\ \hline 0 & 0 & 0 & 0 & \gamma & 2\gamma & \delta_7 & 0 & \alpha+2\beta \\ 0 & 0 & 0 & \gamma & 0 & 2\gamma & 0 & \delta_8 & \alpha+2\beta \\ \hline 0 & 0 & 0 & 0 & 0 & 0 & 2\gamma & 2\gamma & \delta_9 \end{array}\right),$$

where the lines correspond to the blocks in (SM4.3). Here $\delta_i$ is the negative of the sum of the off diagonal elements in the $i$th row of the matrix, so for example $\delta_2 = -(3\alpha + 2\beta + \gamma)$.

**SM5. Lumped generator for two cell vertex-partitions.** While it was easy to compute $\mathbf{q}$ in our example using $\mathbf{Q}$, $\mathbf{C}$ and $\mathbf{D}$, this will not be the case for large systems of interest. Thus we need to consider how we could compute $\mathbf{q}$ without using $\mathbf{Q}$, $\mathbf{C}$ and $\mathbf{D}$ directly. We will use the square example to illustrate this process. For finite $M$ and $P = 2$, a lumped state will be denoted by a matrix $\mathbf{s} \in \mathbb{Z}_{\geq 0}^{M\times P}$ whose $m,p$th entry, $\mathbf{s}_{m,p}$, is the number of vertices in vertex-state $\mathcal{W}_m$ in the vertex partition cell $V_p$.

**SM5.1. Lumped generator for an arbitrary two cell vertex-partition.** We will start by considering the transition rate from an arbitrary lumped state $\mathbf{s}^{[i]}$ to another arbitrary lumped state $\mathbf{s}^{[j]} \neq \mathbf{s}^{[i]}$. In general this is given by

$$\mathbf{q}_{ij} = \frac{1}{|\mathcal{S}_i|} \sum_{S^{[k]}\in\mathcal{S}_i} \sum_{S^{[l]}\in\mathcal{S}_j} \mathbf{Q}_{kl}, \tag{SM5.1}$$

but it turns out that rather than summing over microstates, as (SM5.1) suggests, it is easier to consider the possible transitions of individual vertices and sum their rates.

Let $d_p^v$ denote the number of neighbours of vertex $v$ in the $p$th vertex-partition cell. In our example, all vertices have one neighbour in their own cell and one in the other cell, so $d_1^v = d_2^v = 1$ for all vertices $v$. The degree of vertex $v$ is

$$d^v := \sum_{p=1}^{P} = d_p^v. \tag{SM5.2}$$

We represent the neighbourhood of $v$ using a two-by-two, non-negative, integer-valued matrix $\mathbf{n}^v \in \mathbb{Z}_{\geq 0}^{M\times P}$, whose component $\mathbf{n}_{m,p}^v$ is the number of neighbours of vertex $v$ in the $m$th vertex-state and in the $p$th vertex-partition cell. We call $\mathbf{n}^v$ a *neighbourhood count* and it must satisfy

$$\sum_{m=1}^{M} \mathbf{n}_{m,p}^v = d_p^v,$$

for $0 \leq p \leq P$. Note that

$$\sum_{p=1}^{P} \sum_{m=1}^{M} \mathbf{n}_{m,p}^v = d^v. \tag{SM5.3}$$

We will use a single index on this matrix to indicate a column, i.e. $\mathbf{n}^v_p \in \mathbb{Z}^M_{\geq 0}$ is the $p$th column of $\mathbf{n}^v$.

For our square example, since $d^v_p = 1$ for all $v$ and $p$, the only possibly neighbourhoods in vertex-partition cell $p$ are

$$\begin{pmatrix} 1 \\ 0 \end{pmatrix} \quad \text{and} \quad \begin{pmatrix} 0 \\ 1 \end{pmatrix}, \tag{SM5.4}$$

i.e. either a susceptible or an infected neighbour respectively. Thus the possible neighbourhood counts $\mathbf{n}^v$ are

$$\begin{pmatrix} 1 & 1 \\ 0 & 0 \end{pmatrix}, \begin{pmatrix} 0 & 1 \\ 1 & 0 \end{pmatrix}, \begin{pmatrix} 1 & 0 \\ 0 & 1 \end{pmatrix} \text{ and } \begin{pmatrix} 0 & 0 \\ 1 & 1 \end{pmatrix}. \tag{SM5.5}$$

The first of these matrices corresponds to having a susceptible neighbour in both partitions, the second corresponds to having an infected neighbour in $V_1$ and a susceptible neighbour in $V_2$, and so on.

Without loss of generality we assume that the transition from the lumped state $\mathbf{s}^{[i]}$ to the lumped state $\mathbf{s}^{[j]}$ corresponds to a vertex in vertex-partition $q \in \{1, 2\}$ transitioning from vertex-state $\mathcal{A} \in \mathcal{W}$ to $\mathcal{B} \in \mathcal{W}$, where $\mathcal{A} \neq \mathcal{B}$. To compute (SM5.1), for each $v \in V_q$ we can construct all possible microstates where $v$ has vertex-state $\mathcal{A}$. If in this process we specify the vertex-states of the neighbours of $v$, then we can determine the rate at which $v$ changes from $\mathcal{A}$ to $\mathcal{B}$. Summing this contribution from all possible cases yields $\mathbf{q}_{ij}$. A proof of this is given in Section 6 of the main paper.

The number of ways that we can arrange the vertex-states of the neighbours of $v$ in vertex-partition cell $p \neq q$ according to some $\mathbf{n}^v_p$, as well as the vertex-states of the other vertices in vertex-partition cell $p \neq q$ according to $\mathbf{s}_p$ is

$$A(\mathbf{s}_p, \mathbf{n}^v_p) := \binom{\sum_{p=1}^P \mathbf{n}_{m,p}}{\mathbf{n}^v_p} \binom{\sum_{p=1}^P \mathbf{s}_{m,p} - \mathbf{n}^v_{m,p}}{\mathbf{s}_p - \mathbf{n}^v_p}. \tag{SM5.6}$$

Note that we have used a vector in the bottom of the multinomial coefficient notation to indicate that the elements of the vector should be in the denominator of the multinomial coefficient, i.e.

$$\binom{d^v_p}{\mathbf{n}^v_p} := \frac{d^v_p!}{\mathbf{n}^v_{1,p}!\mathbf{n}^v_{2,p}! \dots \mathbf{n}^v_{m,p}!}.$$

We will also assume the standard convention that a multinomial coefficient is zero if any entry is negative. For the vertex-partition cell $q$, which contains $v$, the number of ways that we can arrange the neighbours of $v$ according to $\mathbf{n}^v_q$ is

$$A(\mathbf{s}_q - \mathbf{e}_{\mathcal{A}}, \mathbf{n}^v_q) = \binom{d^v_q}{\mathbf{n}^v_q} \binom{N_q - 1 - d^v_q}{\mathbf{s}_q - \mathbf{e}_{\mathcal{A}} - \mathbf{n}^v_q},$$

where $\mathbf{e}_{\mathcal{A}}$ is a vector of length $M$ with a one in the entry corresponding to vertex-state $\mathcal{A}$ and zeros elsewhere. This is to account for the fact that we assumed vertex $v$ is in vertex-state $\mathcal{A}$, so there is one less $\mathcal{A}$ vertex in $\mathbf{s}_q$. Then for a given $\mathbf{n}^v$ and $p \neq q$, using (SM5.6) there are

$$A(\mathbf{s}^{[i]}_q - \mathbf{e}_{\mathcal{A}}, \mathbf{n}^v_q) A(\mathbf{s}^{[i]}_p, \mathbf{n}^v_p) \tag{SM5.7}$$

microstates in $\mathcal{S}_i$ in which vertex $v$ in vertex partition cell $q$ is in vertex-state $\mathcal{A}$, its neighbours' vertex-states correspond to $\mathbf{n}^v$, and the total number of vertices in each vertex-state and in each vertex-partition cell corresponds to $\mathbf{s}^{[i]}$. Thus we get $\mathbf{q}_{ij}$ by summing over all feasible realisations of the matrix $\mathbf{n}^v$ and vertices in $V_q$, which yields (SM5.8)

$$\mathbf{q}_{ij} = \frac{1}{\binom{N}{\mathbf{s}^{[i]}}} \sum_{v \in V_q} \sum_{\mathbf{n}_1^v | d_1^v} \sum_{\mathbf{n}_2^v | d_2^v} \left( \zeta_0^{\mathcal{A},\mathcal{B}} + \sum_{m=1}^{M} \sum_{r=1}^{P} \zeta_m^{\mathcal{A},\mathcal{B}} \mathbf{n}_{m,r}^v \right) A(\mathbf{s}_q^{[i]} - \mathbf{e}_{\mathcal{A}}, \mathbf{n}_q^v) A(\mathbf{s}_p^{[i]}, \mathbf{n}_p^v).$$

In this equation, the sums over $\mathbf{n}_1^v | d_1^v$ and $\mathbf{n}_2^v | d_2^v$ specify the $P = 2$ columns of $\mathbf{n}^v$.

For our square example and the case where a transition from $\mathbf{s}^{[i]}$ to $\mathbf{s}^{[j]}$ corresponds to a susceptible vertex in vertex-partition cell $V_1$ becoming infected, (SM5.8) becomes

$$\text{(SM5.9)} \qquad \mathbf{q}_{ij} = \frac{1}{\binom{N}{\mathbf{s}^{[i]}}} \sum_{v \in V_1} \sum_{\mathbf{n}_1^v | d_1^v} \sum_{\mathbf{n}_2^v | d_2^v} \left[ \alpha + \beta \left( \mathbf{n}_{2,1}^v + \mathbf{n}_{2,2}^v \right) \right] A(\mathbf{s}_1 - \mathbf{e}_1, \mathbf{n}_1^v) A(\mathbf{s}_2, \mathbf{n}_2^v).$$

Here $\mathbf{n}_1^v | d_1^v$ corresponds to a sum over non-negative vectors $\mathbf{n}_1^v$ whose elements sum to $d_1^v$, and similarly for $\mathbf{n}_2^v | d_2^v$—in both cases these are the vectors listed in (SM5.4). The lumped states from which a susceptible vertex in $V_1$ can become infected are $\mathbf{S}^{[2]}$, $\mathbf{S}^{[3]}$, $\mathbf{S}^{[5]}$, $\mathbf{S}^{[6]}$ and $\mathbf{S}^{[7]}$. We will use (SM5.9) to compute the lumped transition rate for two examples. First consider the rate from $\mathbf{s}^{[3]}$ to $\mathbf{s}^{[6]}$. For either vertex in $V_1$, expanding the sums over neighbourhoods yields

$$\begin{aligned}
&\sum_{\mathbf{n}_1^v | d_1^v} \sum_{\mathbf{n}_2^v | d_2^v} \left[ \alpha + \beta \left( \mathbf{n}_{2,1}^v + \mathbf{n}_{2,2}^v \right) \right] A(\mathbf{s}_1 - \mathbf{e}_1, \mathbf{n}_1^v) A(\mathbf{s}_2, \mathbf{n}_2^v) \\
=& [\alpha + \beta(0+0)] A\left( \begin{pmatrix} 2 \\ 0 \end{pmatrix} - \begin{pmatrix} 1 \\ 0 \end{pmatrix}, \begin{pmatrix} 1 \\ 0 \end{pmatrix} \right) A\left( \begin{pmatrix} 1 \\ 1 \end{pmatrix}, \begin{pmatrix} 1 \\ 0 \end{pmatrix} \right) \\
&+ [\alpha + \beta(0+1)] A\left( \begin{pmatrix} 2 \\ 0 \end{pmatrix} - \begin{pmatrix} 1 \\ 0 \end{pmatrix}, \begin{pmatrix} 1 \\ 0 \end{pmatrix} \right) A\left( \begin{pmatrix} 1 \\ 1 \end{pmatrix}, \begin{pmatrix} 0 \\ 1 \end{pmatrix} \right) \\
&+ [\alpha + \beta(1+0)] A\left( \begin{pmatrix} 2 \\ 0 \end{pmatrix} - \begin{pmatrix} 1 \\ 0 \end{pmatrix}, \begin{pmatrix} 0 \\ 1 \end{pmatrix} \right) A\left( \begin{pmatrix} 1 \\ 1 \end{pmatrix}, \begin{pmatrix} 1 \\ 0 \end{pmatrix} \right) \\
&+ [\alpha + \beta(1+1)] A\left( \begin{pmatrix} 2 \\ 0 \end{pmatrix} - \begin{pmatrix} 1 \\ 0 \end{pmatrix}, \begin{pmatrix} 0 \\ 1 \end{pmatrix} \right) A\left( \begin{pmatrix} 1 \\ 1 \end{pmatrix}, \begin{pmatrix} 0 \\ 1 \end{pmatrix} \right), \\
=& \alpha \cdot 1 \cdot 1 + [\alpha + \beta] \cdot 1 \cdot 1 + [\alpha + \beta] \cdot 0 \cdot 1 + [\alpha + 2\beta] \cdot 0 \cdot 1, \\
=& 2\alpha + \beta.
\end{aligned}$$

Since there are two vertices in $V_1$, we get a contribution of $2\alpha + \beta$ from each, but the averaging constant is

$$\binom{N}{\mathbf{s}^{[3]}} := \binom{N}{\mathbf{s}_1^{[3]}} \binom{N}{\mathbf{s}_2^{[3]}} = 2,$$

thus we have $\mathbf{q}_{3,6} = 2\alpha + \beta$, which agrees with the corresponding entry in (SM4.4). A similar calculation for the transition from $\mathbf{s}^{[6]}$ to $\mathbf{s}^{[8]}$ yields

$$\begin{aligned}
\mathbf{q}_{6,8} = \frac{1}{4} \times 2 \times \{ &[\alpha + \beta(0+0)] \cdot 0 \cdot 1 + [\alpha + \beta(0+1)] \cdot 0 \cdot 1 \\
&+ [\alpha + \beta(1+0)] \cdot 1 \cdot 1 + [\alpha + \beta(1+1)] \cdot 1 \cdot 1 \} = \alpha + \frac{3}{2}\beta,
\end{aligned}$$

which again agrees with the corresponding entry in (SM4.4).

**SM6. Sum-product property.**

THEOREM SM6.1. *The* sum-product property *is that*

$$\prod_{p=1}^{P}\sum_{i_p=1}^{r_p} a^p_{i_p} = \sum_{i_1=1}^{r_1}\sum_{i_2=1}^{r_2}\cdots\sum_{i_P=1}^{r_P}\prod_{p=1}^{P} a^p_{i_p}.$$

*Proof.* We prove this by induction. This is trivially true for $P=1$. We assume it is true for $P$, then for $P+1$ we have

$$\begin{aligned}\prod_{p=1}^{P+1}\sum_{i_p=1}^{r_p} a^p_{i_p} &= \left(\prod_{p=1}^{P}\sum_{i_p=1}^{r_p} a^p_{i_p}\right)\left(\sum_{i_{P+1}=1}^{r_{P+1}} a^{P+1}_{i_{P+1}}\right),\\ &= \left(\sum_{i_1=1}^{r_1}\sum_{i_2=1}^{r_2}\cdots\sum_{i_P=1}^{r_P}\prod_{p=1}^{P} a^p_{i_p}\right)\left(\sum_{i_{P+1}=1}^{r_{P+1}} a^{P+1}_{i_{P+1}}\right),\\ &= \sum_{i_{P+1}=1}^{r_{P+1}} a^{P+1}_{i_{P+1}}\left(\sum_{i_1=1}^{r_1}\sum_{i_2=1}^{r_2}\cdots\sum_{i_P=1}^{r_P}\prod_{p=1}^{P} a^p_{i_p}\right),\\ &= \sum_{i_1=1}^{r_1}\sum_{i_2=1}^{r_2}\cdots\sum_{i_{P+1}=1}^{r_{P+1}}\prod_{p=1}^{P+1} a^p_{i_p}.\end{aligned}$$ ∎

As a consequence of the sum-product property, for lumped state $\mathbf{s}$ and neighbourhood count $\mathbf{n}^v$ of a vertex $v \in V$, we have

$$\begin{aligned}\prod_{p=1}^{P}\left[\sum_{\mathbf{n}^v_p|d^v_p} A(\mathbf{s}_p,\mathbf{n}^v_p)\right] &= \sum_{\mathbf{n}^v_1|d^v_1}\sum_{\mathbf{n}^v_2|d^v_2}\cdots\sum_{\mathbf{n}^v_P|d^v_P}\prod_{p=1}^{P} A(\mathbf{s}_p,\mathbf{n}^v_p)\\ &= \sum_{\mathbf{n}^v|d^v}\prod_{p=1}^{P} A(\mathbf{s}_p,\mathbf{n}^v_p).\end{aligned} \tag{SM6.1}$$

**SM7. Generalised Vandermonde identity.** The Vandermonde identity can be generalised to multinomials. To see this, consider the multinomial theorem,

$$(x_1+x_2+\cdots+x_M)^N = \sum_{s_1+s_2+\cdots+s_M=N}\binom{N}{s_1,s_2,\ldots,s_M}\prod_{m=1}^{M} x_m^{s_m},$$

where $s_1, s_2, \ldots, s_M \geq 0$. Thus for $d < N$ we have

$$\begin{aligned}&(x_1+x_2+\cdots+x_M)^{N-d}(x_1+x_2+\cdots+x_M)^d\\ &= \left[\sum_{l_1+l_2+\cdots+l_M=N-d}\binom{N-d}{l_1,l_2,\ldots,l_m}\prod_{m=1}^{M} x_m^{l_m}\right]\\ &\qquad\times\left[\sum_{n_1+n_2+\cdots+n_M=d}\binom{d}{n_1,n_2,\ldots,n_M}\prod_{m=1}^{M} x_m^{n_m}\right],\\ &= \sum_{l_1+l_2+\cdots+l_M=N-d}\ \sum_{n_1+n_2+\cdots+n_M=d}\binom{d}{n_1,n_2,\ldots,n_M}\binom{N-d}{l_1,l_2,\ldots,l_m}\prod_{m=1}^{M} x_m^{l_m+n_m},\end{aligned}$$

where $l_m, n_m \geq 0$. Thus instead of summing over $l_1 + l_2 + \cdots + l_M = N - d$ we can sum over $s_1 + s_2 + \cdots + s_M = N$ and use $l_m = s_m - n_m$ with the convention that the multinomial coefficients are zero if $s_m - n_m < 0$ or $\sum_m (s_m - n_m) \neq N - d$. Thus we have

$$\sum_{s_1+s_2+\cdots+s_M=N} \binom{N}{s_1, s_2, \ldots, s_M} \prod_{m=1}^{M} x_m^{s_m} =$$
$$\sum_{s_1+s_2+\cdots+s_M=N} \left[ \sum_{n_1+n_2+\cdots+n_M=d} \binom{d}{n_1, n_2, \ldots, n_M} \binom{N-d}{s_1 - n_1, s_2 - n_2, \ldots, s_M - n_M} \right] \times \prod_{m=1}^{M} x_m^{s_m},$$

and the equality of the polynomials on the two sides implies that the coefficients of corresponding terms are identical, hence

$$\binom{N}{s_1, s_2, \ldots, s_M} = \sum_{n_1+n_2+\cdots+n_M=d} \binom{d}{n_1, n_2, \ldots, n_M} \binom{N-d}{s_1 - n_1, s_2 - n_2, \ldots, s_M - n_M}.$$

LEMMA SM7.1. *Let* $\mathbf{s}$ *be a lumped state and* $\mathbf{n}^v$ *a neighbourhood count of a vertex* $v \in V$*, then*

$$\binom{N}{\mathbf{s}} = \sum_{\mathbf{n}^v | d^v} \prod_{p=1}^{P} A(\mathbf{s}_p, \mathbf{n}_p^v). \tag{SM7.1}$$

*Proof.* From the Vandermonde property of multinomials and (SM5.6), we have

$$\binom{N_p}{\mathbf{s}_p} = \sum_{\mathbf{n}_p^v | d_p^v} A(\mathbf{s}_p, \mathbf{n}_p^v).$$

Thus it follows that

$$\binom{N}{\mathbf{s}} = \prod_{p=1}^{P} \binom{N_p}{\mathbf{s}_p} = \prod_{p=1}^{P} \left( \sum_{\mathbf{n}_p^v | d_p^v} A(\mathbf{s}_p, \mathbf{n}_p^v) \right).$$

The result then follows from application of the sum product property. ∎

**SM8. Degree-based mean-field.** In this section we show that the Eames and Keeling degree-based mean-field is equivalent to the Pastor-Satorras and Vespignani [SM5] degree-based mean-field. The Eames and Keeling degree-based mean-field is

$$\frac{d[I^k]}{dt} = -\gamma [I^k] + \beta \sum_{k'} \frac{[S^k]}{N_k} \frac{[I^{k'}]}{N_{k'}} [kk'], \tag{SM8.1}$$

where $[I^k]$ ($[S^k]$) denotes the number of infected (susceptible) nodes with $k$ neighbours, $N_k$ is the number of nodes with degree $k$, $[kk']$ is the number of partnerships between

individuals with $k$ and $k'$ partners, $\gamma$ is the recovery rate and $\beta$ is the infection rate. Pastor-Satorras and Vespignani use $\rho_k$ to denote the "average density" of infected nodes of degree $k$. The average fraction of infected nodes is then

$$\rho = \sum_k p_k \rho_k,$$

which suggests that $\rho_k = [I^k]/N_k$. The evolution of $\rho_k$ is described by

$$\dot{\rho}_k = -\rho_k + \lambda k \left[1 - \rho_k\right] \frac{\sum_{k'} k' p_{k'} \rho_{k'}}{z}, \tag{SM8.2}$$

where $\lambda = \beta/\gamma$ is the effective spreading rate, and $z = \sum_k k p_k$ is the mean degree. Boguñá et al [SM1] extend this to account for degree correlations, where they define $P(k'|k)$ to be the conditional probability that a node of degree $k$ is connected to a node of degree $k'$. The evolution of $\rho_k$ is then given by

$$\dot{\rho}_k = -\rho_k + \lambda k \left[1 - \rho_k\right] \sum_{k'} P(k'|k) \rho_{k'}. \tag{SM8.3}$$

Now starting from the Ealing and Keemes degree-based mean field, we set $\rho_k = [I^k]/N_k$, so with $N_k = [S^k] + [I^k]$ we have $(1 - \rho_k) = [S^k]/N_k$, then dividing (SM8.1) through by $N_k$ yields

$$\dot{\rho}_k = -\gamma \rho_k + \beta \left[1 - \rho_k\right] \sum_{k'} \frac{[kk']}{N_k} \rho_{k'}.$$

Since $kN_k$ is the total number of edges connected to nodes of degree $k$, we define

$$P(k'|k) = \frac{[kk']}{kN_k},$$

and hence

$$\dot{\rho}_k = -\gamma \rho_k + \beta k \left[1 - \rho_k\right] \sum_{k'} P(k'|k) \rho_{k'},$$

which after time-rescaling yields (SM8.3). In the absence of degree correlations we have

$$P(k'|k) = \frac{k' N_{k'}}{zN} = \frac{k' p_{k'}}{z},$$

and hence we obtain (SM8.2).

## REFERENCES

[SM1] M. Boguná, R. Pastor-Satorras, and A. Vespignani, *Absence of epidemic threshold in scale-free networks with degree correlations*, Physical review letters, 90 (2003), p. 028701.

[SM2] P. Buchholz, *Exact and ordinary lumpability in finite markov chains*, Journal of Applied Probability, 31 (1994), pp. 59–75.

[SM3] J. G. Kemeny, J. L. Snell, et al., *Finite Markov Chains*, vol. 356, van Nostrand Princeton, NJ, 1960.

[SM4] M. Kijima, *Markov processes for stochastic modeling*, vol. 6, CRC Press, 1997.

[SM5] R. Pastor-Satorras and A. Vespignani, *Epidemic spreading in scale-free networks*, Physical Review Letters, 86 (2001), p. 3200.

[SM6] J. A. Ward and M. López-García, *Exact analysis of summary statistics for continuous-time discrete-state markov processes on networks using graph-automorphism lumping*, Applied Network Science, 4 (2019), p. 108.
